# Supplementary material for: MOrdReD: Memory-based Ordinal Regression Deep Neural Networks for Time Series Forecasting
Source: arXiv:1803.09704 source file (2018-10-24)
Supplement: Supplementary file 1 [file appendix_tables.tex]

\begin{table*}[!h]
\centering\begin{tabular}{lrrrr}
\toprule
{} &     \textbf{MOrdReD} &      \textbf{Best GP} &     \textbf{AR(p)} &  \textbf{Seq2Seq regression} \\
\midrule
\textbf{AS\_s3.2\_} &  \textbf{1,067.0291} &   1,459.8154 &  1,154.4474 &          1,148.4572 \\
\textbf{CM\_air.s} &  1,647.5834 &   1,747.9861 &  \textbf{1,300.4001} &          5,490.6812 \\
\textbf{CM\_lwtla} & -\textbf{1,678.6070 }&   1,450.3402 &  1,449.5522 &          7,615.6543 \\
\textbf{CM\_prate} & \textbf{-1,857.4666} &   1,704.9511 &  1,632.7339 &         12,773.7439 \\
\textbf{CM\_rhum1} &    \textbf{674.6915} &   1,505.7443 &  1,415.9282 &          2,952.0419 \\
\textbf{CM\_slp19} &  1,450.5504 &   \textbf{1,385.1744} &  1,432.9088 &          4,218.5500 \\
\textbf{EM\_henon} &  \textbf{1,327.4453} &   1,435.1775 &  1,438.2578 &          1,445.6591 \\
\textbf{EM\_rossl} &    896.0987 &    \textbf{-892.0153} &  1,184.9238 &          1,165.5323 \\
\textbf{EMexptqp} &  1,216.7753 &    \textbf{ 432.4752} &  1,393.8399 &          1,378.7560 \\
\textbf{EMlorenz} &  1,591.2022 &     \textbf{121.5318} &  1,373.5663 &          1,357.3732 \\
\textbf{FI\_yahoo} &  \textbf{1,199.2036} &   1,278.7070 &  1,275.6439 &          4,873.6909 \\
\textbf{FL\_ACT\_L} &  3,208.1393 &   2,697.9846 &  \textbf{1,319.7379} &          1,738.1959 \\
\textbf{FL\_chen\_} & \textbf{ 1,338.2304} &   1,382.0458 &  1,410.6686 &          1,440.1776 \\
\textbf{FL\_dblsc} &  3,950.2313 &   9,972.5421 &  \textbf{1,184.7026} &          5,146.1878 \\
\textbf{FL\_hadle} & -1,299.9369 &  \textbf{-1,475.3231} &  1,186.5957 &          1,322.2664 \\
\textbf{FL\_labyr} &  5,146.8124 & 147,438.9667 &   \textbf{ 276.0968} &         24,374.2497 \\
\textbf{FL\_moore} &  \textbf{1,227.1144} &   1,260.6459 &  1,404.3013 &          1,454.9362 \\
\textbf{FL\_noseh} &  1,597.5401 &   2,593.2756 &  1,347.5664 &          \textbf{1,251.4174} \\
\textbf{FL\_ruckl} &  5,883.6799 &  11,849.8276 &  \textbf{1,348.7245} &          1,943.1374 \\
\textbf{FL\_simpq} &    849.7241 &     \textbf{422.4309} &  1,364.1362 &          1,138.5684 \\
\textbf{FL\_thoma} &  1,640.3127 &   1,734.6156 & \textbf{ 1,411.1365} &          1,590.3507 \\
\textbf{FL\_windm} &  1,274.1142 &     \textbf{667.4089} &  1,319.0198 &          1,400.5067 \\
\textbf{K\_standa} &  \textbf{1,074.6649} &   1,440.4257 &  1,134.9302 &         29,788.0239 \\
\textbf{MC\_inttr} & \textbf{-1,467.4769} &   1,372.3784 &  1,045.9586 &         30,051.7516 \\
\textbf{MP\_Lozi\_} &  \textbf{1,389.3785} &   1,443.7876 &  1,430.1584 &          1,445.1244 \\
\textbf{MP\_freit} &    \textbf{544.8592} &   1,439.2089 &  1,438.4814 &          1,738.2226 \\
\textbf{MP\_logis} & -4,955.7417 &  -3,700.6026 & -\textbf{5,814.7114} &           -639.4380 \\
\textbf{MUS.3\_78} &    \textbf{920.0800} &   1,390.8033 &  1,359.8414 &         25,326.5354 \\
\textbf{MUS\_Si\_l} &  1,232.7973 &   \textbf{1,194.7616} &  1,223.9410 &          2,804.7069 \\
\textbf{SFX\_mach} &  \textbf{1,461.8245} &   1,549.1978 &  1,508.8975 &          1,726.2633 \\
\textbf{SF\_Acont} &    \textbf{875.0483} &   1,825.6995 &  1,343.4891 &          1,342.5143 \\
\textbf{SF\_B1\_1 } &  2,551.0437 &   \textbf{1,784.4138} &  1,808.9434 &          3,106.4496 \\
\textbf{SF\_D1   } &  2,232.7716 &   1,711.1560 &  \textbf{1,588.1358} &          1,594.8293 \\
\textbf{SL\_perci} &  1,205.1593 &   1,088.5775 &  1,122.7930 &            \textbf{993.8790} \\
\textbf{SPIDR\_hp} &    \textbf{685.5992} &   1,621.4097 &  1,650.6923 &          3,572.2350 \\
\textbf{SY\_AR2\_T} &  1,410.4564 &   1,505.1960 &  \textbf{1,399.2487} &          1,508.9031 \\
\textbf{SY\_NLAR2} & \textbf{ 1,378.5653} &   1,419.7959 &  1,421.6656 &          1,418.8368 \\
\textbf{TSAR\_eqe} &    \textbf{493.5048} &     812.4271 &    887.1088 &          1,229.8399 \\
\textbf{TXT\_slc\_} & \textbf{ 1,035.6897} &   1,533.3507 &  1,559.1041 &         28,889.8597 \\
\textbf{AIRFLOW     } &    \textbf{435.9626} &   2,877.8574 &    968.6876 &          4,062.9142 \\
\textbf{ECG   } &    \textbf{296.9145} &   1,287.2807 &  1,396.4655 &          1,686.4036 \\
\textbf{MACKEY      } &  1,030.1611 &     \textbf{-76.3993} &  1,359.9969 &          1,274.3958 \\
\textbf{TIDE    } &  1,480.2779 &     \textbf{965.8456} &  1,726.2864 &          1,921.4516 \\
\textbf{CM\_air.2} &  2,536.3782 &  \textbf{ 1,181.4982} &  1,332.4977 &          7,671.7171 \\
\textbf{CM\_slp2} &  \textbf{1,057.9162} &   1,209.9395 &  1,376.0466 &          1,785.7876 \\
\midrule
\textbf{\# BEST} & \textbf{22} & 12 & 9 & 2 \\
\bottomrule
\end{tabular}
\caption{Negative log-likelihood results for each task in our comparison. Bold indicates best performance.}
\label{tab:nll}
\end{table*}

\begin{table*}
\centering\begin{tabular}{lrrrr}
\toprule
{} &         \textbf{MOrdReD} &         \textbf{Best GP} &         \textbf{AR(p)} &  \textbf{Seq2Seq regression} \\
\midrule
\textbf{AS\_s3.2\_} &    \textbf{537,774.4303} &    730,981.8145 &    583,011.5281 &        602,465.2528 \\
\textbf{CM\_air.s} &    797,310.6650 &    849,920.6264 &    \textbf{595,495.7490} &      1,987,045.6585 \\
\textbf{CM\_lwtla} &   \textbf{-850,655.8811} &    720,115.9146 &    720,560.3084 &      3,475,892.3598 \\
\textbf{CM\_prate} &   \textbf{-962,237.3511 }&    827,452.5737 &    785,376.8963 &                 inf \\
\textbf{CM\_rhum1} &    \textbf{318,715.9516} &    744,527.6240 &    698,875.1607 &      1,318,162.9271 \\
\textbf{CM\_slp19} &    708,956.4100 &    \textbf{676,033.2488} &    708,960.3911 &      1,956,641.3486 \\
\textbf{EM\_henon} &    \textbf{666,538.0935} &    721,627.8115 &    722,434.2246 &        723,671.5397 \\
\textbf{EM\_rossl} &    234,903.2250 &   \textbf{-799,240.1479} &    525,264.2650 &        501,136.6900 \\
\textbf{EMexptqp} &    603,202.4272 &    \textbf{233,318.5896} &    679,917.5012 &        666,458.9532 \\
\textbf{EMlorenz} &    670,342.9368 &   \textbf{-352,288.8058} &    660,739.2650 &        633,814.4291 \\
\textbf{FI\_yahoo} &    \textbf{610,691.1827} &    649,524.6865 &    652,466.7529 &      2,614,821.6856 \\
\textbf{FL\_ACT\_L} &  1,695,738.3760 &    \textbf{202,184.7444} &    549,821.0016 &        859,863.9075 \\
\textbf{FL\_chen\_} &    \textbf{643,972.9990} &    676,464.0209 &    702,070.4431 &        712,645.4365 \\
\textbf{FL\_dblsc} &  1,409,267.6864 &  3,042,435.3927 &    \textbf{319,559.1536} &      1,735,099.8819 \\
\textbf{FL\_hadle} &   -745,731.6830 &   \textbf{-808,478.2369} &    499,370.7651 &        584,166.1370 \\
\textbf{FL\_labyr} &  2,547,025.4252 & 69,599,173.1705 &      \textbf{7,320.5750} &     11,599,495.0842 \\
\textbf{FL\_moore} &    594,250.9651 &     \textbf{-7,825.3522} &    651,279.9919 &        703,499.4243 \\
\textbf{FL\_noseh} &    733,863.0047 &  1,138,630.1639 &    647,597.9971 &        \textbf{576,340.7909} \\
\textbf{FL\_ruckl} &  3,393,325.7608 & 10,305,030.9636 &    \textbf{728,687.1003} &      1,329,705.1824 \\
\textbf{FL\_simpq} &    425,452.2854 &    \textbf{-28,921.5661} &    643,127.8427 &        503,836.9318 \\
\textbf{FL\_thoma} &    755,466.7192 &  1,073,910.4948 &    \textbf{721,636.0546} &        884,462.5645 \\
\textbf{FL\_windm} &    655,510.6083 &    \textbf{-38,691.8916} &    625,721.8445 &        675,112.2497 \\
\textbf{K\_standa} &    \textbf{521,541.7705} &    705,862.8774 &    552,889.6520 &                 inf \\
\textbf{MC\_inttr} &   \textbf{-806,169.2474} &    681,920.7753 &    519,199.8999 &                 inf \\
\textbf{MP\_Lozi\_} &    \textbf{698,082.8050} &    725,860.1243 &    717,822.7702 &        725,154.9156 \\
\textbf{MP\_freit} &    \textbf{282,108.1122} &    716,132.1565 &    717,761.9419 &        861,123.8000 \\
\textbf{MP\_logis} & -2,479,885.5644 & -1,851,887.0580 &\textbf{ -2,937,775.4474} &       -320,044.5399 \\
\textbf{MUS.3\_78} &    \textbf{587,264.6338} &    768,461.1508 &    777,514.2591 &                 inf \\
\textbf{MUS\_Si\_l} &    605,535.4407 &    \textbf{580,569.8597} &    606,199.7606 &      1,374,118.9098 \\
\textbf{SFX\_mach} &    \textbf{738,330.9757} &    816,355.9923 &    787,286.3754 &        952,185.4458 \\
\textbf{SF\_Acont} &    \textbf{326,603.3728} &    737,650.1336 &    652,492.9545 &        639,344.9043 \\
\textbf{SF\_B1\_1 } &  1,043,778.6835 &    \textbf{817,815.9938} &    820,812.0451 &      1,262,284.0170 \\
\textbf{SF\_D1   } &  1,210,384.2928 &    891,784.8620 &    817,067.0744 &        \textbf{793,949.7534} \\
\textbf{SL\_perci} &    582,674.3975 &    514,702.6692 &    532,024.9111 &        \textbf{459,786.5193} \\
\textbf{SPIDR\_hp} &    \textbf{326,188.7176} &    804,120.4900 &    806,853.5498 &      1,803,166.5588 \\
\textbf{SY\_AR2\_T} &    \textbf{680,901.30}34 &    726,950.4163 &    682,292.9675 &        739,537.1911 \\
\textbf{SY\_NLAR2} &    \textbf{696,355.5456} &    712,570.8552 &    712,999.7485 &        712,314.2880 \\
\textbf{TSAR\_eqe} &    \textbf{282,982.3398} &    408,908.6070 &    445,354.1036 &        671,606.1725 \\
\textbf{TXT\_slc\_} &    \textbf{478,537.9735} &    737,348.5886 &    739,450.4873 &                 inf \\
\textbf{AIRFLOW     } &     \textbf{20,871.6061} &  1,108,695.5051 &    377,589.0708 &      1,974,141.3918 \\
\textbf{ECG   } &    \textbf{202,695.9998} &    570,928.6210 &    689,755.1049 &        734,267.2988 \\
\textbf{MACKEY      } &    438,812.5133 &   \textbf{-555,196.3603} &    658,548.5846 &        626,990.6156 \\
\textbf{TIDE    } &    586,436.9008 &    \textbf{378,848.8970} &    790,991.9692 &        933,903.8497 \\
\textbf{CM\_air.2} &    897,901.4183 &    \textbf{546,902.5979} &    640,305.1495 &      2,829,558.4052 \\
\textbf{CM\_slp2} &    \textbf{426,658.4964} &    561,996.3921 &    661,139.2537 &        831,550.6513 \\
\midrule
\textbf{\# BEST} & \textbf{22} & 14 & 6 & 3 \\
\bottomrule
\end{tabular}
    \caption{Integrated negative log-likelihood results for each task in our comparison. Bold indicates best performance.}
    \label{tab:cumnll}
\end{table*}

\begin{table*}
\centering\begin{tabular}{lrrrr} 
\toprule
{} &  \textbf{MOrdReD} &  \textbf{Best GP} &  \textbf{AR(p)} &  \textbf{Seq2Seq regression} \\
\midrule
\textbf{AS\_s3.2\_} &   \textbf{0.0066} &   0.0211 &   0.0096 &              0.0073 \\
\textbf{CM\_air.s} &   0.0295 &   0.0170 &  \textbf{ 0.0014} &              0.0748 \\
\textbf{CM\_lwtla} &   0.0110 &   \textbf{0.0066} &   0.0075 &              0.0906 \\
\textbf{CM\_prate} &   0.2647 &   0.0554 &   \textbf{0.0549} &              0.2777 \\
\textbf{CM\_rhum1} &   0.0103 &   0.0166 &   \textbf{0.0078} &              0.0347 \\
\textbf{CM\_slp19} &   0.0042 &   0.0007 &   \textbf{0.0006} &              0.0587 \\
\textbf{EM\_henon} &   \textbf{0.0001} &   0.0023 &   0.0029 &              0.0026 \\
\textbf{EM\_rossl} &   0.0024 &   0.0032 &   0.0005 &              \textbf{0.0002} \\
\textbf{EMexptqp} &   0.0023 &   0.0080 &   \textbf{0.0007} &              0.0042 \\
\textbf{EMlorenz} &   0.0024 &   0.0062 &   \textbf{0.0003} &              0.0021 \\
\textbf{FI\_yahoo} &  \textbf{ 0.0009} &   0.0032 &   0.0025 &              0.0225 \\
\textbf{FL\_ACT\_L} &   0.0611 &   0.0196 &   \textbf{0.0112} &              0.0802 \\
\textbf{FL\_chen\_} &   0.0001 &   \textbf{5.01e-5} &   0.0009 &              0.0018 \\
\textbf{FL\_dblsc} &   0.0340 &   0.0489 &   \textbf{0.0020} &              0.0593 \\
\textbf{FL\_hadle} &   0.0084 &   0.0028 &   \textbf{0.0016} &              0.0065 \\
\textbf{FL\_labyr} &   0.3317 &   0.3317 &   \textbf{0.0512} &              0.3316 \\
\textbf{FL\_moore} &   \textbf{0.0023} &   0.0040 &   0.0033 &              0.0062 \\
\textbf{FL\_noseh} &   0.0065 &   0.0440 &   \textbf{0.0006} &              0.0007 \\
\textbf{FL\_ruckl} &   \textbf{0.0076} &   0.0132 &   0.0170 &              0.1098 \\
\textbf{FL\_simpq} &   \textbf{0.0002} &   0.0003 &   0.0018 &              0.0004 \\
\textbf{FL\_thoma} &   0.0328 &   0.0041 &   \textbf{0.0041} &              0.0165 \\
\textbf{FL\_windm} &   \textbf{0.0007} &   0.0136 &   0.0035 &              0.0062 \\
\textbf{K\_standa} &   \textbf{0.0012} &   0.0179 &   0.0055 &              0.0756 \\
\textbf{MC\_inttr} &   0.2047 &   0.0550 &   \textbf{0.0520} &              0.2041 \\
\textbf{MP\_Lozi\_} &   \textbf{0.0002} &   0.0005 &   0.0007 &              0.0007 \\
\textbf{MP\_freit} &   \textbf{0.0004} &   0.0116 &   0.0125 &              0.0386 \\
\textbf{MP\_logis} &   0.3004 &   \textbf{0.0453} &   0.0527 &              0.0498 \\
\textbf{MUS.3\_78} &   \textbf{0.0059} &   0.0230 &   0.0203 &              0.0649 \\
\textbf{MUS\_Si\_l} &   0.0021 &   0.0019 &   \textbf{0.0012} &              0.0306 \\
\textbf{SFX\_mach} &   \textbf{3.78e-5} &   0.0009 &   0.0006 &              0.0056 \\
\textbf{SF\_Acont} &   \textbf{0.0036} &   0.0198 &   0.0052 &              0.0056 \\
\textbf{SF\_B1\_1 } &   0.0301 &   \textbf{0.0011} &   0.0021 &              0.0194 \\
\textbf{SF\_D1   } &   0.0362 &   0.0376 &   0.0163 &              \textbf{0.0140} \\
\textbf{SL\_perci} &   0.0266 &   \textbf{0.0013} &   0.0059 &              0.0016 \\
\textbf{SPIDR\_hp} &   \textbf{0.0021} &   0.0253 &   0.0156 &              0.0657 \\
\textbf{SY\_AR2\_T} &   \textbf{0.0011} &   0.0041 &   0.0024 &              0.0135 \\
\textbf{SY\_NLAR2} &   0.0027 &   0.00014 &   \textbf{0.0001} &              0.0006 \\
\textbf{TSAR\_eqe} &   \textbf{0.0079} &   0.0201 &   0.0235 &              0.0123 \\
\textbf{TXT\_slc\_} &   \textbf{0.0003} &   0.0100 &   0.0061 &              0.0870 \\
\textbf{AIRFLOW     } &   0.0048 &   0.0633 &  \textbf{ 0.0042} &              0.0711 \\
\textbf{ECG   } &   0.0431 &   0.0622 &   0.0328 &             \textbf{ 0.0183} \\
\textbf{MACKEY      } &   \textbf{0.0005} &   0.0011 &   0.0023 &              0.0027 \\
\textbf{TIDE    } &   0.0645 &   0.1086 &   \textbf{0.0142} &              0.0253 \\
\textbf{CM\_air.2} &   0.0231 &   0.0243 &   \textbf{0.0086} &              0.0954 \\
\textbf{CM\_slp2} &   0.0110 &   \textbf{0.0008} &   0.0018 &              0.0212 \\
\midrule
\textbf{\# BEST} & \textbf{18} & 6 & 18 & 3 \\
\bottomrule
\end{tabular}
    \caption{Euclidean distance between the identity function and the reliability plot for each task in our comparison. Bold indicates best performance.}
    \label{tab:qq}
\end{table*}

\begin{table*}
\centering\begin{tabular}{lrrrr}
\toprule
{} &  \textbf{MOrdReD} &  \textbf{Best GP} &  \textbf{AR(p)} &  \textbf{Seq2Seq regression} \\
\midrule
\textbf{AS\_s3.2\_} &   \textbf{0.0094} &   0.0235 &   0.0122 &              0.0300 \\
\textbf{CM\_air.s} &   0.0169 &   0.0541 &   \textbf{0.0048} &              0.0728 \\
\textbf{CM\_lwtla} &   \textbf{0.0061} &   0.0085 &   0.0080 &              0.0568 \\
\textbf{CM\_prate} &   0.2856 &   0.0575 &   \textbf{0.0567} &              0.2890 \\
\textbf{CM\_rhum1} &   \textbf{0.0012} &   0.0016 &   0.0013 &              0.0185 \\
\textbf{CM\_slp19} &   0.0055 &   \textbf{0.0017} &   0.0045 &              0.0678 \\
\textbf{EM\_henon} &   \textbf{0.0002} &   0.0022 &   0.0021 &              0.0019 \\
\textbf{EM\_rossl} &   0.0123 &   0.0502 &   0.0040 &              \textbf{0.0030} \\
\textbf{EMexptqp} &   0.0053 &   0.0443 &   \textbf{0.0009} &              0.0086 \\
\textbf{EMlorenz} &   0.0056 &   0.0097 &   \textbf{0.0013} &              0.0056 \\
\textbf{FI\_yahoo} &   \textbf{0.0005} &   0.0020 &   0.0013 &              0.0262 \\
\textbf{FL\_ACT\_L} &   0.2183 &   \textbf{0.0180} &   0.0245 &              0.1056 \\
\textbf{FL\_chen\_} &   \textbf{0.0004} &   0.0007 &   0.0013 &              0.0009 \\
\textbf{FL\_dblsc} &   0.1264 &   0.1586 &  \textbf{ 0.0593} &              0.2006 \\
\textbf{FL\_hadle} &   0.0034 &   0.0035 &   \textbf{0.0011} &              0.0105 \\
\textbf{FL\_labyr} &   0.3317 &   0.3317 &   \textbf{0.0540} &              0.3314 \\
\textbf{FL\_moore} &   0.0163 &   \textbf{0.0058} &   0.0101 &              0.0171 \\
\textbf{FL\_noseh} &   0.0069 &   0.0374 &   \textbf{0.0007} &              0.0007 \\
\textbf{FL\_ruckl} &   0.1852 &   0.1319 &   \textbf{0.0236} &              0.1248 \\
\textbf{FL\_simpq} &   0.0110 &   0.0072 &   \textbf{0.0005} &              0.0033 \\
\textbf{FL\_thoma} &   0.1390 &   0.1033 &   \textbf{0.1021} &              0.2193 \\
\textbf{FL\_windm} &   \textbf{0.0014} &   0.0294 &   0.0037 &              0.0054 \\
\textbf{K\_standa} &   \textbf{0.0036} &   0.0153 &   0.0060 &              0.0779 \\
\textbf{MC\_inttr} &   0.2329 &   \textbf{0.0604} &   0.0614 &              0.2397 \\
\textbf{MP\_Lozi\_} &   \textbf{0.0004} &   0.0006 &   0.0007 &              0.0007 \\
\textbf{MP\_freit} &   \textbf{0.0018} &   0.0069 &   0.0068 &              0.0261 \\
\textbf{MP\_logis} &   0.2977 &   \textbf{0.0443} &   0.0525 &              0.0489 \\
\textbf{MUS.3\_78} &   0.0039 &   0.0013 &   \textbf{0.0005} &              0.0770 \\
\textbf{MUS\_Si\_l} &   \textbf{0.0003} &   0.0006 &   0.0024 &              0.0457 \\
\textbf{SFX\_mach} &   \textbf{0.0006} &   0.0082 &   0.0044 &              0.0156 \\
\textbf{SF\_Acont} &   0.0097 &   \textbf{0.0068} &   0.0070 &              0.0080 \\
\textbf{SF\_B1\_1 } &   0.0069 &   0.0041 &   0.0053 &              \textbf{0.0017} \\
\textbf{SF\_D1   } &   0.0576 &   0.0528 &   0.0239 &              \textbf{0.0078} \\
\textbf{SL\_perci} &   0.0543 &   0.0280 &   0.0246 &              \textbf{0.0153} \\
\textbf{SPIDR\_hp} &   \textbf{0.0006} &   0.0264 &   0.0153 &              0.0557 \\
\textbf{SY\_AR2\_T} &   \textbf{0.0025} &   0.0069 &   0.0042 &              0.0173 \\
\textbf{SY\_NLAR2} &   0.0151 &   \textbf{0.0054} &   0.0065 &              0.0135 \\
\textbf{TSAR\_eqe} &   \textbf{0.0065} &   0.0227 &   0.0250 &              0.0082 \\
\textbf{TXT\_slc\_} &   \textbf{0.0054} &   0.0280 &   0.0192 &              0.1169 \\
\textbf{AIRFLOW     } &   0.1135 &   0.2125 &   \textbf{0.0126} &              0.0559 \\
\textbf{ECG   } &   0.0812 &   0.0361 &   0.0335 &              \textbf{0.0108} \\
\textbf{MACKEY      } &   0.0036 &   0.0079 &   \textbf{0.0013} &              0.0037 \\
\textbf{TIDE    } &   0.1674 &   0.1899 &   \textbf{0.0283} &              0.0594 \\
\textbf{CM\_air.2} &   \textbf{0.0171} &   0.0644 &   0.0376 &              0.0809 \\
\textbf{CM\_slp2} &   \textbf{0.0023} &   0.0045 &   0.0071 &              0.0210 \\
\midrule
\textbf{\# BEST} & \textbf{18} & 7 & 15 & 5 \\
\bottomrule
\end{tabular}
    \caption{Euclidean distance between the identity function and the reliability plot for each task in our comparison. Reliability plots for this table were computed from only the first 250 out-f-sample predictions generated by each model for each dataset. Bold indicates best performance.}
    \label{tab:qq250}
\end{table*}

\begin{table*}
\centering\begin{tabular}{lrrrr}
\toprule
{} &  \textbf{MOrdReD} &  \textbf{Best GP} &  \textbf{AR(p)} &  \textbf{Seq2Seq regression} \\
\midrule
\textbf{AS\_s3.2\_} &   1.8147 &   1.5639 &   1.6351 &              \textbf{1.3664} \\
\textbf{CM\_air.s} &   \textbf{1.0681} &   1.5650 &   1.4570 &              1.3134 \\
\textbf{CM\_lwtla} &   \textbf{1.4926} &   1.7521 &   1.8053 &              1.5809 \\
\textbf{CM\_prate} &   \textbf{0.7965} &   1.4023 &   1.4006 &              1.9711 \\
\textbf{CM\_rhum1} &   \textbf{1.1057} &   1.5822 &   1.6819 &              1.4002 \\
\textbf{CM\_slp19} &   1.5448 &   1.6020 &   1.7388 &              \textbf{1.3921} \\
\textbf{EM\_henon} &   \textbf{1.3646} &   1.7034 &   1.7747 &              1.7425 \\
\textbf{EM\_rossl} &   0.7428 &  \textbf{ 0.2904} &   1.1970 &              1.2620 \\
\textbf{EMexptqp} &   1.0935 &   \textbf{0.6750} &   1.7299 &              1.5902 \\
\textbf{EMlorenz} &   1.5430 &   \textbf{0.9303} &   1.6717 &              1.5241 \\
\textbf{FI\_yahoo} &   \textbf{1.6647} &   1.6732 &   1.6885 &              1.8315 \\
\textbf{FL\_ACT\_L} &   \textbf{0.9427} &   1.1732 &   1.6232 &              1.5676 \\
\textbf{FL\_chen\_} &   \textbf{1.4854} &   1.6635 &   1.7470 &              1.6514 \\
\textbf{FL\_dblsc} &   1.5428 &   1.4025 &   \textbf{1.1624} &              1.3952 \\
\textbf{FL\_hadle} &   0.7312 &   \textbf{0.1298} &   1.2714 &              1.5234 \\
\textbf{FL\_labyr} &   0.7911 &   1.9941 &   \textbf{0.0353} &              1.0676 \\
\textbf{FL\_moore} &   1.5840 &   \textbf{1.1501} &   1.6711 &              1.5540 \\
\textbf{FL\_noseh} &   1.4959 &   \textbf{1.2923} &   1.6407 &              1.5371 \\
\textbf{FL\_ruckl} &   1.5515 &   \textbf{1.1251} &   1.5250 &              1.5019 \\
\textbf{FL\_simpq} &   0.7904 &   \textbf{0.7676} &   1.5257 &              1.2256 \\
\textbf{FL\_thoma} &   \textbf{1.2368} &   1.4740 &   1.7531 &              1.4419 \\
\textbf{FL\_windm} &   1.3481 &  \textbf{ 0.9162} &   1.6585 &              1.6944 \\
\textbf{K\_standa} &   1.6337 &   \textbf{1.5711} &   1.6532 &              1.8597 \\
\textbf{MC\_inttr} &   \textbf{0.3040} &   1.4128 &   1.5416 &              1.7998 \\
\textbf{MP\_Lozi\_} &   \textbf{1.5819} &   1.7303 &   1.7244 &              1.7612 \\
\textbf{MP\_freit} &   \textbf{1.3093} &   1.7869 &   1.8015 &              1.6288 \\
\textbf{MP\_logis} &   \textbf{0.0000} &   0.0008 &   0.0002 &              0.0304 \\
\textbf{MUS.3\_78} &   1.7685 &   \textbf{1.5454} &   1.5610 &              1.7256 \\
\textbf{MUS\_Si\_l} &   1.8375 &   1.6673 &   1.7280 &              \textbf{1.3604} \\
\textbf{SFX\_mach} &   1.9651 &   \textbf{1.6139} &   1.6852 &              1.7161 \\
\textbf{SF\_Acont} &   \textbf{1.0772} &   1.5164 &   1.6801 &              1.7120 \\
\textbf{SF\_B1\_1 } &   1.4776 &   1.6354 &   1.7227 &              \textbf{1.4735} \\
\textbf{SF\_D1   } &   1.4701 &   1.5502 &   1.7781 &              \textbf{1.1392} \\
\textbf{SL\_perci} &   \textbf{1.1529} &   1.5393 &   1.5464 &              1.2299 \\
\textbf{SPIDR\_hp} &   \textbf{1.1855} &   1.6951 &   1.6681 &              1.6401 \\
\textbf{SY\_AR2\_T} &   1.7251 &   1.7359 &   1.7413 &             \textbf{ 1.5590} \\
\textbf{SY\_NLAR2} &   \textbf{1.5561} &   1.7345 &   1.7044 &              1.7295 \\
\textbf{TSAR\_eqe} &   1.5632 &   1.5945 &   \textbf{1.5434} &              1.8148 \\
\textbf{TXT\_slc\_} &   \textbf{1.1753} &   1.7161 &   1.7330 &              1.9347 \\
\textbf{AIRFLOW     } &   \textbf{0.5783} &   1.4398 &   1.1710 &              1.3795 \\
\textbf{ECG   } &   \textbf{0.8779} &   1.7244 &   1.5423 &              1.3119 \\
\textbf{MACKEY      } &   \textbf{0.8303} &   0.9571 &   1.6755 &              1.1923 \\
\textbf{TIDE    } &   0.6660 &   \textbf{0.5474} &   1.5541 &              1.7027 \\
\textbf{CM\_air.2} &   1.1996 &   \textbf{1.0856} &   1.6023 &              1.3777 \\
\textbf{CM\_slp2} &   \textbf{0.8115} &   1.4028 &   1.6949 &              1.6707 \\
\midrule
\textbf{\# BEST} & \textbf{22} & 14 & 3 & 6 \\
\bottomrule
\end{tabular}
    \caption{Symmetric mean absolute percentage error between the out-of-sample ground truth and the median of the predictive distribution in each task. Bold indicates best performance.}
    \label{tab:smape}
\end{table*}

\begin{table*}
\centering\begin{tabular}{lrrrr}
\toprule
{} &  \textbf{MOrdReD} &  \textbf{Best GP} &  \textbf{AR(p)} &  \textbf{Seq2Seq regression} \\
\midrule
\textbf{AS\_s3.2\_} &   \textbf{0.5426} &   0.5727 &   0.5589 &              0.5541 \\
\textbf{CM\_air.s} &   \textbf{3.0849} &   4.5161 &   3.4446 &              4.5771 \\
\textbf{CM\_lwtla} &   1.5717 &   \textbf{1.3109} &   1.3224 &              1.4851 \\
\textbf{CM\_prate} &   \textbf{1.0638} &   1.4032 &   1.3341 &              1.5605 \\
\textbf{CM\_rhum1} &   1.7210 &   1.7658 &   1.7015 &              \textbf{1.6697} \\
\textbf{CM\_slp19} &   1.9858 &   \textbf{1.7761} &   1.8697 &              2.0328 \\
\textbf{EM\_henon} &   \textbf{0.5991} &   0.6167 &   0.6240 &              0.6236 \\
\textbf{EM\_rossl} &   4.8200 &   \textbf{1.7475} &   6.8972 &              7.1416 \\
\textbf{EMexptqp} &   9.6667 &   \textbf{4.8841} &  15.0529 &             14.8472 \\
\textbf{EMlorenz} &  15.9257 &  \textbf{10.1526} &  17.9497 &             16.5222 \\
\textbf{FI\_yahoo} &   0.5512 &   0.5510 &   0.5525 &              \textbf{0.5454} \\
\textbf{FL\_ACT\_L} &  32.4316 &  \textbf{23.8210} &  30.9129 &             46.5224 \\
\textbf{FL\_chen\_} &   \textbf{1.2572} &   1.3243 &   1.3327 &              1.3513 \\
\textbf{FL\_dblsc} &  75.3228 &  64.7602 &  \textbf{53.9632} &             76.6752 \\
\textbf{FL\_hadle} &   4.9416 &   \textbf{0.5291} &   8.1644 &              9.4631 \\
\textbf{FL\_labyr} & 115.2523 & 203.5818 &  \textbf{ 7.4167} &            141.4771 \\
\textbf{FL\_moore} &  15.9446 &  \textbf{10.6950} &  15.9200 &             15.9541 \\
\textbf{FL\_noseh} &   1.8345 &   1.7576 &   1.4722 &              \textbf{1.3791} \\
\textbf{FL\_ruckl} &  63.8383 &  \textbf{39.2245} &  40.9307 &             61.2674 \\
\textbf{FL\_simpq} &   2.4511 &   \textbf{2.3188} &   3.7916 &              3.1231 \\
\textbf{FL\_thoma} &  23.2105 &  19.7964 &  \textbf{19.0195} &             20.5371 \\
\textbf{FL\_windm} &  10.4500 &   \textbf{8.7484} &  10.3780 &             10.5306 \\
\textbf{K\_standa} &   0.6057 &   0.6237 &   0.6089 &             \textbf{ 0.6044} \\
\textbf{MC\_inttr} &   \textbf{0.2462} &   0.7217 &   0.7130 &              0.6629 \\
\textbf{MP\_Lozi\_} &   \textbf{0.5460} &   0.5569 &   0.5547 &              0.5610 \\
\textbf{MP\_freit} &   \textbf{1.6743} &   1.7503 &   1.7561 &              1.8569 \\
\textbf{MP\_logis} &   \textbf{0.0000} &   0.0004 &   0.0001 &              0.0149 \\
\textbf{MUS.3\_78} &   0.4800 &   0.5052 &   0.4977 &              \textbf{0.4785} \\
\textbf{MUS\_Si\_l} &   1.4069 &   1.4068 &   \textbf{1.402}8 &              1.4441 \\
\textbf{SFX\_mach} &   \textbf{0.5429} &   0.5615 &   0.5593 &              0.5549 \\
\textbf{SF\_Acont} &   \textbf{0.8664} &   0.9414 &   1.0149 &              1.0183 \\
\textbf{SF\_B1\_1 } &   4.4003 &   \textbf{4.2859} &   4.3081 &              4.4033 \\
\textbf{SF\_D1   } &   3.4762 &   3.6023 &   \textbf{3.3636} &              3.3687 \\
\textbf{SL\_perci} &   3.0529 &   2.8010 &   2.7753 &              \textbf{2.6506} \\
\textbf{SPIDR\_hp} &  \textbf{ 0.9355} &   1.1215 &   1.0268 &              1.2590 \\
\textbf{SY\_AR2\_T} &   \textbf{3.0317} &   3.0846 &   3.0617 &              3.3181 \\
\textbf{SY\_NLAR2} &   0.8251 &   0.8157 &   \textbf{0.8079} &              0.8165 \\
\textbf{TSAR\_eqe} &   1.2974 &   1.3331 &   1.3262 &              \textbf{1.2815} \\
\textbf{TXT\_slc\_} &   \textbf{0.8972} &   0.9829 &   0.9421 &              0.9351 \\
\textbf{AIRFLOW     } &  \textbf{11.3865} &  24.7673 &  20.3718 &             34.0315 \\
\textbf{ECG   } &   \textbf{1.7155} &   3.2871 &   2.0379 &              1.8861 \\
\textbf{MACKEY      } &   \textbf{4.1942} &   4.5775 &   6.6189 &              5.4394 \\
\textbf{TIDE    } &  16.2222 & \textbf{ 11.6931} &  31.8119 &             32.6614 \\
\textbf{CM\_air.2} &   4.9184 &   \textbf{3.5470} &   4.3098 &              5.4936 \\
\textbf{CM\_slp2} &   \textbf{1.9344} &   2.7490 &   3.1656 &              3.3104 \\
\midrule
\textbf{\# BEST} & \textbf{18} & 14 & 6 & 7 \\
\bottomrule
\end{tabular}
    \caption{Mean absolute scaled error between the out-of-sample ground truth and the median of the predictive distribution in each task. Bold indicates best performance.}
    \label{tab:mase}
\end{table*}
